# Supplementary material for: Greedy Growing Enables High-Resolution Pixel-Based Diffusion Models
Source: arXiv:2405.16759 source file (2024-05-27)
Supplement: Supplementary file 1 [file painting_prompts.tex]

\begin{enumerate}
\itemsep0em 
\scriptsize{
\item 
A photomontage of a businesswoman, peering out of a window, with a city skyline in the background, in the style of 'Mona Lisa' by Leonardo da Vinci.
\item
A group of friends sharing a pizza in the style of 'The Last Supper' by Leonardo da Vinci.	
\item
A vibrant city landscape in the style of 'The Starry Night' by Vincent van Gogh, with swirling lights and soaring skyscrapers.	\item
A portrait featuring a child expressing intense emotion in the style of 'The Scream' by Edvard Munch.	
% \item  "A romantic couple sharing a tender embrace under the depths of the ocean, with the lovers adorned in seaweed and surrounded by shimmering sea creatures in the style of 'The Kiss' by Gustav Klimt, adorned with gold leaf and intricate patterns."
\item Girl With a Glittery Earring in the style of 'Girl With a Pearl Earring' by Johannes Vermeer.	\item
A fashion model photographed as Venus on the shell in the style of 'The Birth of Venus' by Sandro Botticelli.	\item
A portrait of a proud group of pet owners with their beloved dogs in the style of 'Las Meninas' by Diego Velázquez.	\item
A portrait of a scientist holding a plant in the style of 'Creation of Adam' by Michelangelo, highlighting the beauty of the human form and science.	\item
A city skyline at dawn in the style of 'Impression Sunrise' by Claude Monet, with pastel brushstrokes and a hazy, dreamy quality.	\item
A group of friends posing as different characters in the style of 'The Great Wave off Kanagawa' by Hokusai, with bold lines and vibrant colors.	\item
% A melting digital clock placed on a rocky surface in the style of 'The Persistence of Memory' by Salvador Dalí.	\item
A group of friends enjoying a summer day at a riverside restaurant in the style of 'A Sunday Afternoon on the Island of La Grande Jatte' by Georges Seurat.	\item
A portrait of a woman standing on a mountain peak, looking out at the vast landscape in the style of "Wanderer above the Sea of Fog" by Caspar David Friedrich.	\item
% A fresco mural of a modern cityscape with people of different cultures interacting together in the style of 'Sistine Chapel's ceiling' by Michelangelo.	\item
A self-portrait of a bohemian artist in the style of 'Arnolfini Portrait' by Jan van Eyck, with a pronounced use of perspective.	\item
A photograph of a group of friends in a park, dancing and enjoying each other’s company in the style of 'Bal du moulin de la Galette' by Pierre-Auguste Renoir.	\item
A group of modern-day survivors on a life raft with the theme of survival echoing 'The Raft of the Medusa' by Théodore Géricault.	\item
A futuristic school in the style of 'The School of Athens' by Raphael, depicting the gathering of philosophers and scholars containing both humans and aliens.	\item
A satellite falling from the sky in the style of 'Landscape with the Fall of Icarus' by Pieter Bruegel the Elder.	\item
A rooftop garden with colorful lights in the style of 'Café Terrace at Night' by Vincent van Gogh, depicting a dreamy, starry sky.	\item
A realistic painting depicting a surgeon performing surgery in the style of 'The Beheading of St John the Baptist' by Caravaggio.	\item
A modern group enjoying a picnic in the countryside in the style of 'The Harvesters' by Pieter Bruegel the Elder.
% \item
% A painting by Grant Wood of an astronaut couple, american gothic style.	
% \item
% An intricate and imaginative composition in the style of 'Composition 8' by Wassily Kandinsky, resembling an abstract world in shades of blue.
\item
A photograph of a young asian girl on a swing in a lush garden in the style of 'The Swing' by Jean-Honoré Fragonard, conveying a sense of freedom and joy.	\item
A modern, diverse family reunion scene in the style of 'The Return of the Prodigal Son' by Rembrandt.	\item
A beautifully floral romper in the style of 'The Sleeping Gypsy' by Henri Rousseau, surrounded by lush foliage and exotic flowers.	\item
A depiction of volunteers cleaning a beach with Fagaras Mountains in the background in the style of "The Gleaners" by Jean-François Millet.	\item
A baby squirrel with wings being held by his mother in the style of 'The Sistine Madonna' by Raphael.
% \item
% A vibrant and colorful urban streetscape in Singapore in the style of 'The Avenue in the Rain' by Childe Hassam, with reflections on wet pavements.	
\item
A vibrant street scene in Istanbul the style of 'Paris Street; Rainy Day' by Gustave Caillebotte, capturing the reflections of light and movement through the wet pavement.	\item
A portrait of a female subject in a long flowing asian kimono in the style of 'The Lady of Shalott' by John William Waterhouse, capturing the mystical and ethereal atmosphere of the painting.	\item
A lively grocery store scene in the style of 'A Bar at the Folies-Bergère' by Édouard Manet.	\item
A vibrant and lively caribean bar scene in the style of 'The Night Café' by Vincent van Gogh, with warm colors and expressive brushstrokes.	\item
A photograph of high-altitude skydivers in the style of 'Oath of the Horatii' by Jacques-Louis David, capturing the dramatic poses and arrangement of the figures.	\item
A group of construction workers in the style of 'The Night Watch' by Rembrandt.	\item
A vintage-style portrait of a mother sitting beside a miniature train set on a coffee table in the style of 'Whistler's Mother' by James McNeill Whistler.	\item
A mural art showing women in a protective stance alongside men fighting with soldiers in the background, all carrying the Canadian flag, in the style of 'Liberty Leading the People' by Eugène Delacroix.	\item
A group of friends smiling and laughing as they enjoy a relaxing day on a boat in the style of 'Luncheon of the Boating Party.	\item
A dynamic rendition of a racing cyclist leading their team through a mountain pass, rendered in the style of 'Napoleon Crossing the Alps' by Jacques-Louis David.	\item
A desolate scene of a modern ship struggling in a tempestuous sea in the style of 'The Storm on the Sea of Galilee' by Rembrandt.	\item
A freelance photographer crafting her vision in the style of 'The Garden of Earthly Delights' by Hieronymus Bosch.	\item
Capture a bustling freight hub in the heart of a metropolis, complete with towering stacks of shipping containers and bustling cargo operations, in the style of 'A Cotton Office in New Orleans' by Edgar Degas.
% \item
% A digital collage featuring vibrant geometric shapes and swirling patterns in the style of 'Color Study: Squares with Concentric Circles' by Wassily Kandinsky.
% \item A distressed dachshund being comforted by a wise-looking cat in the style of 'A Friend In Need' by Cassius Marcellus Coolidge.
\item
A blossoming almond tree by a calm lake in the style of 'Carnation, Lily, Lily, Rose' by John Singer Sargent.
}
\end{enumerate}
