# Supplementary material for: Greedy Growing Enables High-Resolution Pixel-Based Diffusion Models
Source: arXiv:2405.16759 source file (2024-05-27)
Supplement: Supplementary file 2 [file painting_template.tex]

\begin{table}[tbh!]
\vspace*{-\baselineskip}
\centering
\resizebox{\linewidth}{!}{
\begin{tabular}{ll}
\hline
Template:
\\
\multicolumn{2}{c}{
$ \mathtt{[Description\_o\_the\_subject]}~in~the~style~of~ \mathtt{[Art\_Style\_or\_Artist\_Name]}, \mathtt{[Medium (optional)]},
\mathtt{[Key Visual Elements or Mood (optional)]}
$
}
\\
\hline
Examples: \\
&
Here are some examples to help get you started:
\\
& Caption:~A majestic mountain landscape in the style of Impressionism, Claude Monet, oil painting, hazy atmosphere, soft sunlight.
\\
&Caption:~A portrait of a woman in the style of Art Nouveau, Alphonse Mucha, flowing lines, intricate details, muted color palette.
\\
\hline
Artist: & Name :\\
Mona Lisa	&	Leonardo da Vinci	 \\
The Last Supper	&	Leonardo da Vinci	 \\
The Starry Night	&	Vincent van Gogh	 \\
The Scream	&	Edvard Munch	 \\
% Guernica	&	Pablo Picasso	 \\ % -----04
% The Kiss	&	Gustav Klimt	 \\
Girl With a Pearl Earring	&	Johannes Vermeer	 \\
The Birth of Venus	&	Sandro Botticelli	 \\
Las Meninas	&	Diego Velázquez	 \\
Creation of Adam	&	Michelangelo	 \\
Impression Sunrise	&	Claude Monet	 \\
The Great Wave off Kanagawa	&	Hokusai	 \\
% The Persistence of Memory	&	Salvador Dalí	 \\
A Sunday Afternoon on the Island of La Grande Jatte	&	Georges Seurat	 \\
Wanderer above the Sea of Fog	&	Caspar David Friedrich	 \\
% Sistine Chapel ceiling	&	Michelangelo	 \\
Arnolfini Portrait	&	Jan van Eyck	 \\
% Nude Descending a Staircase, No. 2	&	Marcel Duchamp	 \\
Bal du moulin de la Galette	&	Pierre-Auguste Renoir	 \\
The Raft of the Medusa	&	Théodore Géricault	 \\
The School of Athens	&	Raphael	 \\
Landscape with the Fall of Icarus	&	Pieter Bruegel the Elder	 \\
Café Terrace at Night	&	Vincent van Gogh	 \\
The Beheading of St John the Baptist	&	Caravaggio	 \\
The Harvesters	&	Pieter Bruegel the Elder	 \\
% American Gothic	&	Grant Wood	 \\
% Composition 8	&	Wassily Kandinsky	 \\
The Swing	&	Jean-Honoré Fragonard	 \\
The Return of the Prodigal Son	&	Rembrandt	 \\
The Sleeping Gypsy	&	Henri Rousseau	 \\
The Gleaners	&	Jean-François Millet	 \\
The Sistine Madonna	&	Raphael	 \\
% The Avenue in the Rain	&	Childe Hassam	 \\
Paris Street; Rainy Day	&	Gustave Caillebotte	 \\
The Lady of Shalott	&	John William Waterhouse	 \\
A Bar at the Folies-Bergère	&	Édouard Manet	 \\
The Night Café	&	Vincent van Gogh	 \\
Oath of the Horatii	&	Jacques-Louis David	 \\
% Royal Red and Blue	&	Mark Rothko	 \\
The Night Watch	&	Rembrandt	 \\
Whistler's Mother	&	James McNeill Whistler	 \\
Liberty Leading the People	&	 Eugène Delacroix 	 \\
Luncheon of the Boating Party	&	Pierre-Auguste Renoir	 \\
Napoleon Crossing the Alps	&	Jacques-Louis David	 \\
The Storm on the Sea of Galilee	&	Rembrandt	 \\
The Garden of Earthly Delights	&	Hieronymus Bosch	 \\
A Cotton Office in New Orleans	&	Edgar Degas	 \\
% Color Study: Squares with Concentric Circles	&	Wassily Kandinsky	 \\
% A Friend In Need	&	Cassius Marcellus Coolidge	 \\
Carnation, Lily, Lily, Rose	&	John Singer Sargent	 \\
\hline
\end{tabular}
}
\caption{Template used to create prompts mimicking famous paintings style.}
\label{tab:memorization_template}
\end{table}

\begin{table}
\resizebox{\linewidth}{!}{
\begin{tabular}{|ll|}
\hline
Fields:
\\
\hline
$\mathtt{[Description\_of\_the\_subject]}$: & Describe what you want to be in the image (e.g., a person, a landscape, an object, an abstract concept).
\\
$\mathtt{[Art\_Style\_or\_Artist\_Name]}$: & Specify the art movement or artist you want to emulate (e.g., Impressionism, Claude Monet).
\\
$\mathtt{
[Medium (optional)]}$: &
This is where you can get creative! Indicate if you want the results to look like a medium like oil painting, watercolor, digital art, charcoal sketch, photography, etc.
\\
$\mathtt{
[Key Visual Elements or Mood (optional)]:}$ &
Add additional keywords that describe the atmosphere, mood, lighting, or specific elements you want (e.g., "dreamy," "vibrant," "sunset," "dramatic lighting”).
\\
\hline
\end{tabular}
}
\end{table}
